# Supplementary material for: Perspective-Aware Teaching: Adapting Knowledge for Heterogeneous Distillation
Source: arXiv:2501.08885 source file (2025-10-16)
Supplement: Supplementary file 1 [file X_suppl.tex]

\clearpage
\setcounter{page}{1}
\maketitlesupplementary

\section{Implementation Details}

We follow the training procedure of OFA-KD\cite{hao2023ofa} and employ different training settings for different student models based on their architecture. Specifically, we utilize the SGD optimizer for CNN-based models, whereas we opt for the AdamW optimizer for ViT-based and MLP-based models and additionally incorporate augmentations such as Mixup \cite{zhang2018mixup}, and CutMix \cite{yun2019cutmix}. All models are trained for 300 epochs on CIFAR-100. In the case of ImageNet, CNN-based models are trained for only 100 epochs, while ViT-based and MLP-based student models are trained for 300 epochs.

\section{Lower Effectiveness in CNN-based students}

As shown in the experimental results on CIFAR-100 and ImageNet, PAT yields relatively limited gains on CNN-based student models. We attribute this to limitations of the RAA module. The effectiveness of RAA relies on the overlap between the student’s effective receptive field (ERF) and the global context needed for teacher-student feature alignment. CNNs typically exhibit a Gaussian-shaped ERF, limiting global context coverage and leading to suboptimal feature fusion. Consequently, RAA becomes less effective, as CNN-based students lack sufficient global information in intermediate features for attention-based reblending. While there is no architectural incompatibility as attention is a superset of convolution, CNN-based students may require longer training to benefit from RAA, and future work could explore solutions specifically tailored to this scenario.

% As shown in the experiment tables, our method PAT demonstrates relatively limited improvements on CNN-based student models. We believe this is primarily due to the limitations introduced by the RAA module. The effectiveness of RAA depends on the overlap between the student model’s effective receptive field (ERF) and the global context required for teacher-student feature alignment. CNNs typically have a Gaussian-like ERF, which limits global context coverage and leads to suboptimal feature fusion. As a result, RAA is less effective since the student's intermediate features lack sufficient global information on CNN-based models for attention-based reblending. While there is no architectural incompatibility as attention is a superset of convolution, CNN-based students may require longer training to benefit from RAA, and future work could explore solutions specifically tailored to this scenario.

\section{Distillation in homogeneous architectures}

% \definecolor{Gray}{gray}{0.85}
% \newcolumntype{a}{>{\columncolor{Gray}}c}

\begin{table}[]
    \centering
    \resizebox{\linewidth}{!}{
    % \begin{tabular}{c|cc|cccccccc}
    %      \toprule
    %      & T. & S. & KD & OFD & Review & CRD & DKD & DIST & OFA & OF2\\
    %      \midrule
    %     Accuracy & 73.31 & 69.75 & 70.66 & 70.81 & 71.61 & 71.17 & 71.70 & 72.07 & 72.10 &  \\
    %     \bottomrule
    % \end{tabular}
    \begin{tabular}{c|cc|ccccccc}
         \toprule
        Method & T. & S. & KD & OFA & AT & CRD & PAT \\
         \midrule
        Acc. & 73.31 & 69.75 & 70.66 & \textbf{72.10} & 69.56 & 71.17 & \underline{71.18} \\
        \bottomrule
    \end{tabular}
    }
    \caption{Result on ImageNet with ResNet34 - ResNet18 homogeneous teacher-student model pair. Our results are the average over 3 trials. The highest results are indicated in bold, while the second-best results are underlined.}
    \label{tab:ablation_homo}
    \vspace{-5pt}
\end{table}

We further assess our approach through the distillation of homogenous architectures to validate its generalizability. The results are shown in Table~\ref{tab:ablation_homo}. When distilling from a homogeneous teacher, our method experiences a 1.43\% performance improvement to the student model but has a slight performance drop compared to state-of-the-art OFA. Our proposed module, RAA, is meticulously crafted to reconcile the disparity between the perspectives of the student and teacher models. However, when distilling from models that possess similar perspectives, the efficacy of RAA diminishes, and the incorporation of additional parameters may complicate the training process.

\section{Data efficiency on ViTs in heterogeneous KD}

\begin{table}[]
    \centering
    \begin{tabular}{c|cccc}
    \toprule
         & 25\% & 50\% & 75\% & 100\% \\
    \midrule
        Student & 40.74 & 55.98 & 65.28 & 68.00 \\
        PAT    & 52.23 & 68.21 & 74.58 & 79.59 \\
    \bottomrule
    \end{tabular}
    \caption{Date efficiency experiment result on CIFAR-100 with ConvNeXt-T - DeiT-T teacher-student model pair.}
    \label{tab:ablation_data_efficient}
    \vspace{-5pt}
\end{table}

Vision transformers (ViTs) are known for their data-hungry issue, where they need substantial amounts of data to achieve satisfactory performance. On the other hand, CNNs are capable of attaining commendable performance levels with a comparatively modest volume of data. Consequently, we have devised an experiment aimed at investigating whether a ViT-based student model can attain comparable performance levels using a reduced amount of data, particularly when under the distillation of a data-efficient CNN-based teacher model.

Table~\ref{tab:ablation_data_efficient} illustrates the comparative performance of the naive student model alongside our PAT methodology utilizing varying proportions of the training dataset, specifically 25\%, 50\%, 75\%, and 100\%. It is evident that our PAT consistently surpasses the naive student model. The absence of inductive bias in the ViT-based model makes it challenging to attain favorable performance levels with restricted data, as evidenced by its modest achievement of 40.74\% with merely 25\% of the available data. Nevertheless, the ViT-based model demonstrates a significant enhancement in performance when subjected to distillation from a data-efficient CNN-based teacher, thereby highlighting an additional advantage of heterogeneous knowledge distillation.

% \section{Limitations}

% A limitation of our approach lies in significant memory consumption during training. Our AFP utilizes the prompt tuning technique to adjust the stage feature of the teacher model with minimal parameters, however, this approach necessitates the backward propagation through the teacher model, resulting in substantial memory consumption. One potential solution to this issue could involve replacing the prompt tuning technique in AFP with a more sophisticated parameter-efficient fine-tuning method such as ladder side-tuning\cite{sung2022lst}. We consider this task as our future research to enhance the modification of teacher features more efficiently. 
% that is both efficient in terms of parameters and memory usage.

\begin{table}[]
    \centering
    \begin{tabular}{cccc}
        \toprule
         &  & ConvNeXt-T & ConvNeXt-T \\
        RAA & AFP & DeiT-T & ResMLP-S12 \\
        % RAA & AFP & ConvNeXt-T - DeiT-T & ConvNeXt-T - ResMLP-S12 \\
        \midrule
        \multicolumn{2}{c}{Baseline (FitNet)}   & 60.71 & 45.47 \\
        \midrule
        \checkmark &  & 70.12 & 75.04 \\
         & \checkmark & 73.07 & 80.12 \\
        \checkmark & \checkmark & 79.59 & 83.50 \\
        \bottomrule
    \end{tabular}
    \caption{The effectiveness of RAA, AFP on CIFAR-100.}
    \label{tab:table9}
    \vspace{-10pt}
\end{table}

\section{Ablation of RAA in Table 4}

Table~\ref{tab:table9} shows that removing RAA results in a significant performance drop, confirming its importance. Without RAA, student must rely on single-stage alignment, losing the ability to integrate multi-layer features to bridge the gap with the teacher's representations.

% \bibliography{strings, aaai25}
% \bibliography{strings,ref}

{
    \small
    \bibliographystyle{ieeenat_fullname}
    \bibliography{strings, main}
}

\end{document}
